# Supplementary material for: Phase-field material point method for dynamic brittle fracture with isotropic and anisotropic surface energy
Source: arXiv:1906.04740 source file (2019-06-11)
Supplement: Supplementary file 1 [file Appendix.tex]

\begin{appendices}
\vspace{-6pt}
\section{Strain energy density decomposition} \label{App:SEDD}
\vspace{-2pt}

%====================Strain Energy Density Decomposition ===================================

In Eq. \eqref{eqn:ElasticStrainEnergyDesn}, the strain energy density $\psi_{el}$ is assumed to be additively decomposed into a tensile $\psi_{el}^{+}$ and a compressive part $\psi_{el}^{-}$ as in Miehe et al. \cite{miehe_2010b}. In this, the positive part is expressed as
\begin{equation}
	\psi _{el}^ +  = \frac{1}{2}\lambda {\left\langle {\Tr\left[ \boldsymbol{\varepsilon}  \right]} \right\rangle^{{+}^{2}}} + \mu \Tr\left[ {{{\left( {{\boldsymbol \varepsilon ^ + }} \right)}^2}} \right].
	\label{ElasEnergDensityPlus}
\end{equation}
Similarly, the negative part is expressed as
\begin{equation}
	\psi _{el}^ -  = \frac{1}{2}\lambda {\left\langle {\Tr\left[ \boldsymbol{\varepsilon}  \right]} \right\rangle^{{-}^{2}}} + \mu \Tr\left[ {{{\left( {{\boldsymbol \varepsilon ^ - }} \right)}^2}} \right].
	\label{ElasEnergDensityMinus}
\end{equation}
Parameters $\lambda$ and $\mu$ stand for the Lam\'{e} constants. The symbols $\langle{ . }\rangle^{+}$ and $\langle{ . }\rangle^{-}$ are defined as $\langle{ x}\rangle^{+} = \left( x + |x| \right) /{2}$ and $\langle{x}\rangle^{-} = \left(x - |x| \right) /{2}$, respectively, whereas the symbol $\Tr$ stands for the trace. The positive and the negative part of strain tensor are expressed as
\begin{equation}
	\label{StrainTensPlus}
	{{\boldsymbol \varepsilon ^ + }}= \bm{P} \bm{\Lambda ^ + } \bm{P}^T
\end{equation}
and 
\begin{equation}
	\label{StrainTensMinus}
	\boldsymbol \varepsilon^-=\boldsymbol \varepsilon  - {\boldsymbol \varepsilon ^ + },
\end{equation}
respectively, where $\bm{P}$ is a matrix whose columns comprise the eigen-vectors of the strain tensor $\boldsymbol \varepsilon$ and $\bm{\Lambda ^ + }$ is a diagonal matrix defined as
\begin{equation}
	\label{EigenValues}
	\bm{\Lambda ^ + }=\text{diag}\left(\langle\lambda_1\rangle^{+},\langle\lambda_2\rangle^{+},\langle\lambda_3\rangle^{+}\right)
\end{equation}
where $\lambda_i,i=1,\dots,3$ are the eigen-values of the strain tensor.

\end{appendices}
